# Supplementary material for: Streaming Technologies and Serialization Protocols: Empirical Performance Analysis
Source: arXiv:2407.13494 source file (2024-11-04)
Supplement: Supplementary file 1 [file appendices.tex]

\section{\break Name-1}
Appendix goes here
